# Supplementary material for: Density functional theory based investigation of heavy fermion band candidates in triplet superconductor UTe2
Source: arXiv:2410.03840 ancillary file (2024-10-04)
Supplement: Supplementary file 1 [file SZL_UTe2DFT_SM_10_02.pdf]

# Supplemental Material for: Density functional theory based investigation of heavy fermion band candidates in triplet superconductor $UTe_2$

Shouzheng Liu

(Dated: June 2024)

## I. LINEAR COMBINATION OF ATOMIC ORBITALS (LCAO)

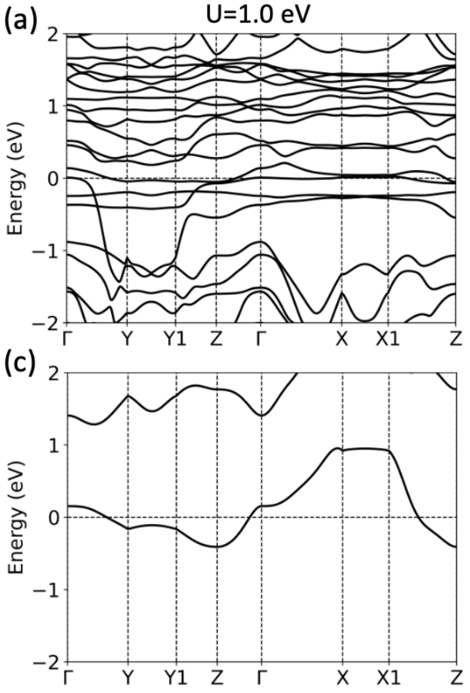


Fig. S1. Full DFT+U band structure for $UTe_2$ calculated using (a) U=1.0 eV and (b) U=1.6 eV. The U-dz$^2$ orbital dispersions, obtained by down-folding to a tight-binding (TB) model and retaining only the hoppings within U-dz$^2$ orbitals, are shown for (c) U=1.0 eV and (d) U=1.6 eV.

Typically, maximally localized Wannier functions (MLWF) are used to construct TB models from *ab initio* calculations[1, 2]. However, to preserve the original orbital symmetry, we opted for the alternative approach of using pure spherical harmonic atomic orbitals with only the radial wavefunction $u_n(r)$ variationally adjusted to maximize overlap with the original band basis[3]:

$$\phi_n(\vec{r}) = u_n(r) Y_{lm}(\hat{r}). \tag{1}$$

These atomic orbitals are used to form a momentum space basis via the corresponding Bloch sums:

$$B_{n,\vec{k}}(\vec{r}) = N^{-\frac{1}{2}} \sum_{\vec{R}} e^{i\vec{k}\cdot\vec{R}} \phi_n(\vec{r} - \vec{R}). \tag{2}$$

The DFT Hamiltonian $H(\vec{k})$ is then projected onto this new atomic orbital basis set:

$$H_{mn}(\vec{k}) = \langle B_{m,\vec{k}} | \, H(\vec{k}) \, | B_{n,\vec{k}} \rangle \, . \tag{3}$$

Finally, the TB Hamiltonian $H(\vec{R})$ is obtained by performing a Fourier transformation on $H(\vec{k})$. As shown in Fig. 1(c) of the main text, this approach faithfully reproduces the DFT band structure.

The DFT+U calculations in Fig. S1 were performed using WIEN2k with the Hubbard potentials U=1.6 eV as in the main text (Fig. S1(b)) and U=1.0 eV (Fig. S1(a))[4]. Due to the difference in parameters, two calculations yielded Fermi surfaces with different topology as reported in earlier research [5]. To test the robustness of our projection for orbital symmetry properties, these *ab initio* calculations are converted into two TB models and the $dz^2$ dispersion is isolated by excluding all other orbitals (Fig. S1(c-d)). The U-$dz^2$ bands from the two calculations are offset in energy relative to the Fermi level due to the dependency of $f$-orbital occupancy on U, but otherwise show similar dispersions that reflect the stability of the orbital-resolved Hamiltonian across the two convergence regimes.

## II. GUTZWILLER-LIKE RENORMALIZATION

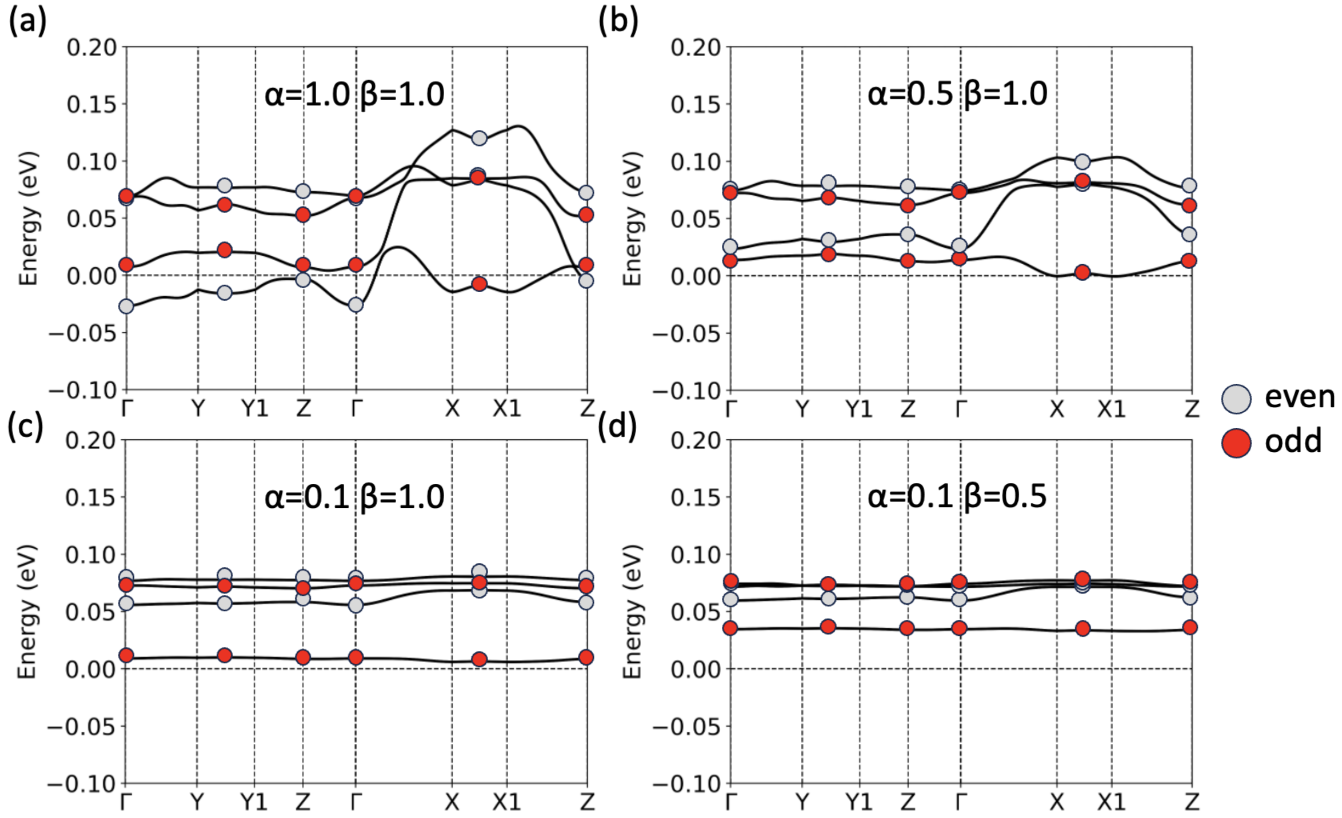


Fig. S2. Dispersion of the TB model projected to a U-5$f$ orbital basis under different renormalization parameters: (a) $\alpha = 1.0$, $\beta = 1.0$; (b) $\alpha = 0.5$, $\beta = 1.0$; (c) $\alpha = 0.1$, $\beta = 1.0$; and (d) $\alpha = 0.1$, $\beta = 0.5$. The even and odd parity states are marked with grey and red circles, respectively. A fixed rectangular contour is used for the X-Y momentum space, for clarity in visualizing the quasi-1D sublattice dispersions. Because of this, some parity labels fall between the labeled momentum coordinates.

In the main text, following Gutzwiller's approximation, all U-5$f$ creation and annihilation operators are renormalized by a factor of $\sqrt{\alpha}$, with the exception that the intra-dimer and same-atom $f \leftrightarrow f$ hamiltonian terms. These are left unchanged to preserve the local orbital energies and to avoid the need for an *ad hoc* term defining the energy offset of $f$ electrons relative to other orbitals. For Fig. S2, the Hamiltonian is projected to an $f$ orbital basis and the intra-dimer $f \leftrightarrow f$ hoppings $t_1$ are controlled by a new parameter $\beta$ to observe the bare $f$-electron dispersions and crystal field energetics. As depicted in Fig. S2(a-c), decreasing $\alpha$ from 1 to 0.1 causes the overall energy-axis width of bands to reduce modestly from $\sim$0.09 to 0.07 eV at the $\Gamma$-point, and mostly eliminates a large ($> 0.1$ eV) band dispersion along the $k_x$ axis ($\Gamma$-X and X1-Z). In Fig. S2(d), the *intra-dimer* hoppings are renormalized, reducing a crystal field gap between the lower even-parity band and the upper band cluster. The intra-dimer hoppings effectively control the splitting between bonding and anti-bonding states of the dimer, with a $\gtrsim$0.05 eV energy scale that is larger than other crystal field effects (note the $\sim$10 meV scale of splitting between higher energy $f$ bands in Fig. S2(d)). These intradimer terms are unchanged ($\beta = 1$) in the main text as noted above.

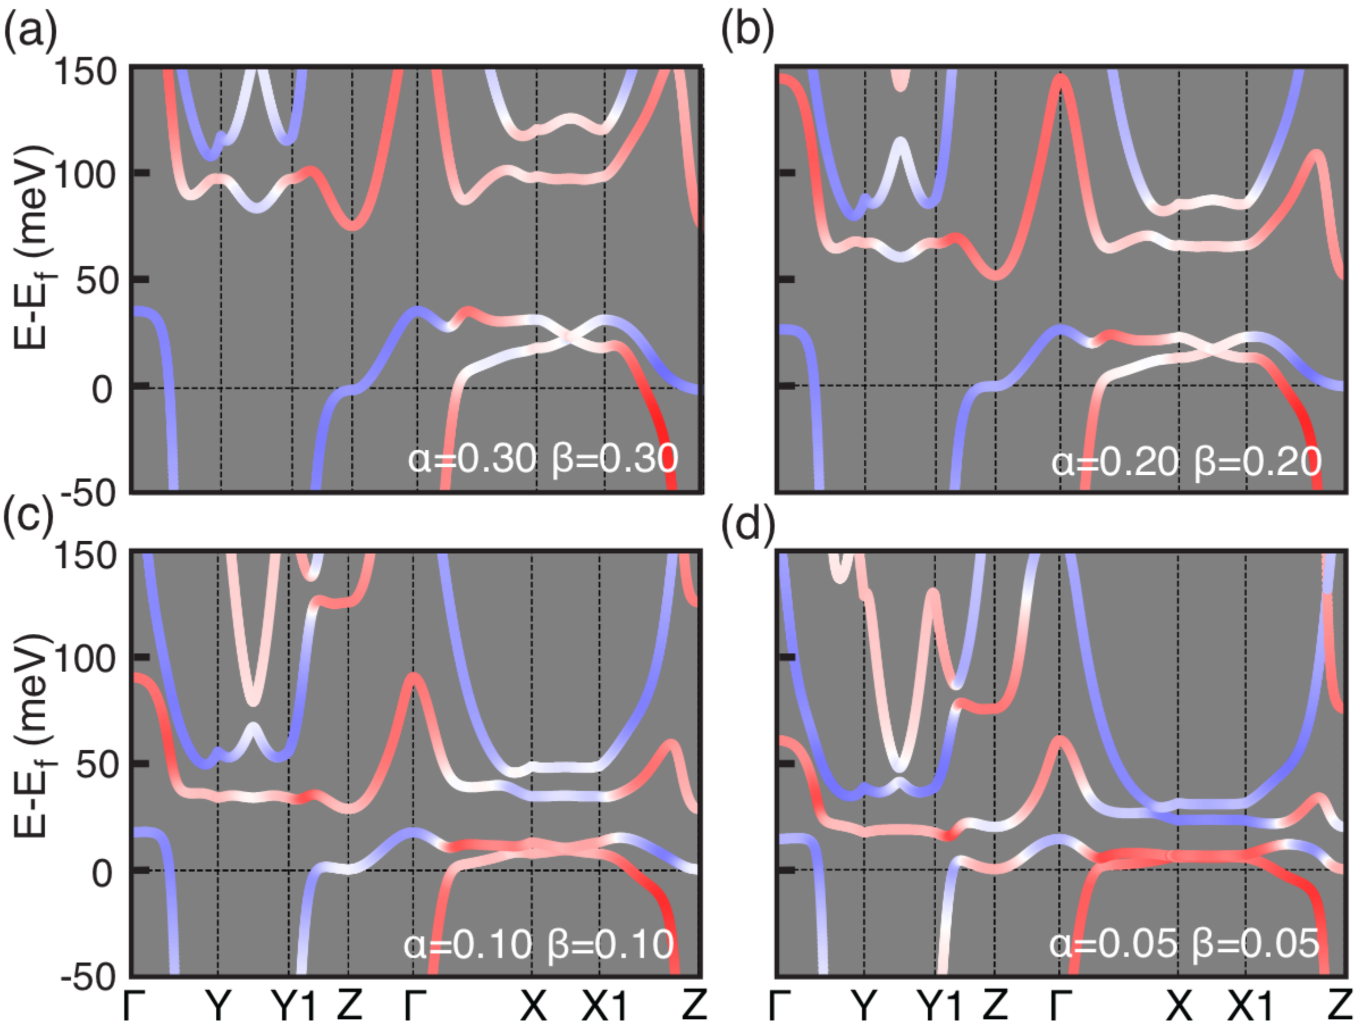


Fig. S3. A uniform renormalization scheme, which includes renormalization for the intra-dimer $f \leftrightarrow f$ hoppings, is applied under varying renormalization parameters: (a) $\alpha = 0.3$; (b) $\alpha = 0.2$; (c) $\alpha = 0.1$; and (d) $\alpha = 0.05$. The shading indicates the relative orbital weight between $f_{xz^2}$ (red) and $f_{y(3x^2-y^2)}$ (blue).

In Fig. S3, we also present band structure calculations based on a renormalization scheme that applies the same renormalization factor of $\sqrt{\alpha}$ to both intra-dimer and inter-dimer f-electron related hoppings in the TB Hamiltonian ($\alpha = \beta$). Our results in the main text remain consistent with this alternative renormalization approach. As the degree of renormalization is increased, the low energy bands remain the same, and parabolicity of the lower $5f_{y(3x^2-y^2)}$ band along the $k_y$ axis reverses sign due to hybridization with the upper $5f_{xz^2}$ band, leading to a transition from a saddle point to a local minimum at the Z-point.

## III. QUANTUM OSCILLATION (QO) AND RESISTIVITY SIMULATIONS

The frequencies observed in QO measurements are proportional to the area of the extremal orbits on the Fermi surfaces. Previous experiments observed a branch of QO signal exhibiting a plateau around $f \sim 3$ kT when rotating towards the $\hat{a}$ axis [7], which deviates from the expected $f \propto cos^{-1}(\theta)$ trend for a tube structure. In Fig. S4 (a-c), we present QO simulations results for the WIEN2k calculation with U=1.6 eV, which shows poorer alignment compared to our renormalized tight-binding (TB) model discussed in the main text. Furthermore, a previous WIEN2k calculation with U=2.0 eV also failed to explain the plateau around 3 kT[7].

For completeness, we also provide a TB model with all U-5$f$ orbitals removed, as shown in Fig. S4 (d-f). This model is similar to the $ThTe_2$ band structure described in Ref. [8], in which $f$-electron states are not found close

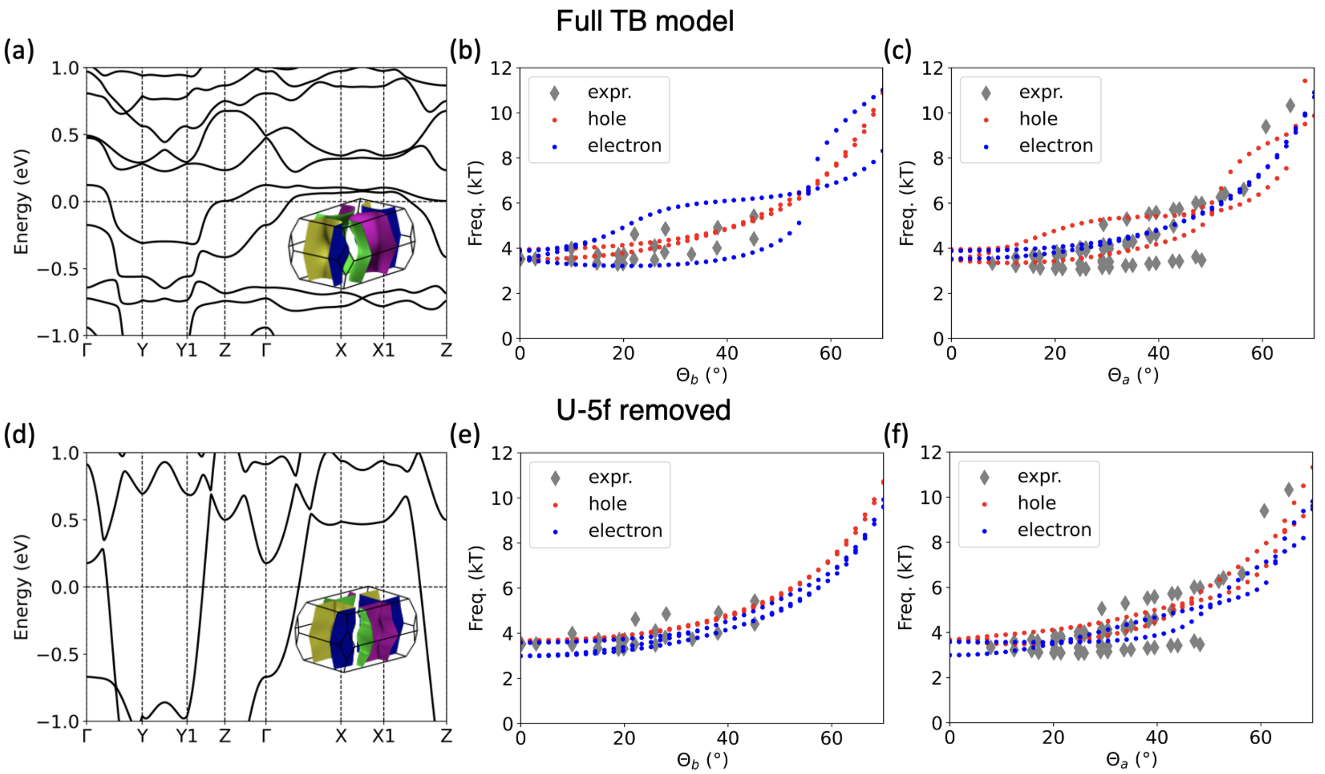


Fig. S4. (a) Band structure from a DFT+U calculation with U=1.6 eV, using WIEN2k. The inset shows the Fermi surfaces. Panels (b) and (c) present quantum oscillation simulations compared with experimental data from Ref. [6] and Ref. [7], respectively. Similar plots for a tight-binding (TB) model with all U-5$f$ orbitals removed are shown in panels (d) to (f).

to the Fermi level. The chemical potential is shifted by 1.13 eV to account for the loss of occupied 5$f$ states and approximate the Fermi wavevectors observed from ARPES. In this TB model, the tube structure is free from the corrugation caused by hybridization with U-5$f$ bands, resulting in a more nearly $f \propto cos^{-1}(\theta)$ trend. Both examples illustrate that the interaction between the light bands and the strongly correlated U-5$f$ bands is crucial for an accurate description of the Fermi surfaces.

It should be noted that the loss of electrons from the light bands when a Z-point Fermi pocket is introduced has negligible impact on the light band QO branches at $\sim 4$ kT. The reason for this is that the Z-point Fermi pocket realized in the main text has an extremely small Luttinger volume of 0.0048 e-/BZ, and may realistically be counted as 0.0024 e-/BZ due to the reduced valence basis of the 5$f$ band.

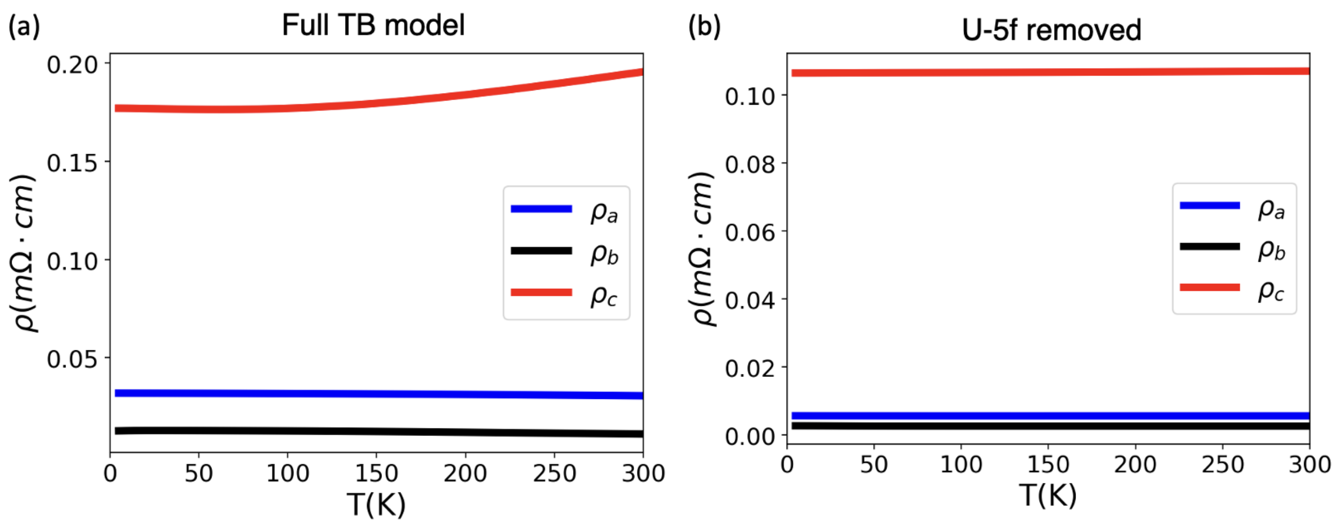


Fig. S5. Resistivity simulations for the DFT+U (U=1.6 eV) model (a) and the TB model without U-5$f$ orbitals (b). Both simulations use a constant scattering strength Γ=4 meV. The resistivities $\rho_a$, $\rho_b$, and $\rho_c$ are represented by blue, black, and red lines, respectively.

The resistivity simulations for these two models are presented in Fig. S5. Using a constant scattering strength, both simulations show $\rho_c \gg \rho_a > \rho_b$, while experimental results indicate $\rho_c \sim \rho_b > \rho_a$[9]. However, it is noticeable in Fig. S5 (a) $\rho_c$ exhibits an upward trend with increasing temperature, similar to the experiment results. This suggests that part of the observed temperature dependence of $\rho_c$ could intrinsically stem from the hybridization between the light bands and the strongly correlated U-5$f$ bands. In contrast, the TB model with all U-5$f$ orbitals removed shows almost linear dispersion near the Fermi level, resulting in flat resistivity as the temperature increases.

[1] D. Gresch, Q. Wu, G. W. Winkler, R. Häuselmann, M. Troyer, and A. A. Soluyanov, Automated construction of symmetrized wannier-like tight-binding models from ab initio calculations, Phys. Rev. Mater. **2**, 103805 (2018).

[2] G. Pizzi, V. Vitale, R. Arita, S. Blügel, F. Freimuth, G. Géranton, M. Gibertini, D. Gresch, C. Johnson, T. Koretsune, J. Ibañez-Azpiroz, H. Lee, J.-M. Lihm, D. Marchand, A. Marrazzo, Y. Mokrousov, J. I. Mustafa, Y. Nohara, Y. Nomura, L. Paulatto, S. Poncé, T. Ponweiser, J. Qiao, F. Thöle, S. S. Tsirkin, M. Wierzbowska, N. Marzari, D. Vanderbilt, I. Souza, A. A. Mostofi, and J. R. Yates, Wannier90 as a community code: new features and applications, Journal of Physics: Condensed Matter **32**, 165902 (2020).

[3] M. Nakhaee, S. A. Ketabi, and F. M. Peeters, Tight-Binding Studio: A technical software package to find the parameters of tight-binding Hamiltonian, Computer Physics Communications **254**, 107379 (2020).

[4] P. Blaha, K. Schwarz, F. Tran, R. Laskowski, G. K. Madsen, and L. D. Marks, WIEN2k: An APW+lo program for calculating the properties of solids, The Journal of chemical physics **152** (2020).

[5] J. Ishizuka, S. Sumita, A. Daido, and Y. Yanase, Insulator-Metal Transition and Topological Superconductivity in $UTe_2$ from a First-Principles Calculation, Phys. Rev. Lett. **123**, 217001 (2019).

[6] A. Eaton, T. Weinberger, N. Popiel, Z. Wu, A. Hickey, A. Cabala, J. Pospíšil, J. Prokleška, T. Haidamak, G. Bastien, *et al.*, Quasi-2D Fermi surface in the anomalous superconductor $UTe_2$, Nature Communications **15**, 223 (2024).

[7] D. Aoki, H. Sakai, P. Opletal, Y. Tokiwa, J. Ishizuka, Y. Yanase, H. Harima, A. Nakamura, D. Li, Y. Homma, *et al.*, First observation of the de Haas–van Alphen effect and Fermi surfaces in the unconventional superconductor $UTe_2$, Journal of the Physical Society of Japan **91**, 083704 (2022).

[8] L. Miao, S. Liu, Y. Xu, E. C. Kotta, C.-J. Kang, S. Ran, J. Paglione, G. Kotliar, N. P. Butch, J. D. Denlinger, *et al.*, Low energy band structure and symmetries of $UTe_2$ from angle-resolved photoemission spectroscopy, Physical review letters **124**, 076401 (2020).

[9] Y. S. Eo, S. Liu, S. R. Saha, H. Kim, S. Ran, J. A. Horn, H. Hodovanets, J. Collini, T. Metz, W. T. Fuhrman, A. H. Nevidomskyy, J. D. Denlinger, N. P. Butch, M. S. Fuhrer, L. A. Wray, and J. Paglione, $c$-axis transport in $UTe_2$: Evidence of three-dimensional conductivity component, Phys. Rev. B **106**, L060505 (2022).
